# Supplementary material for: Whole genome mapping of 5' RNA ends in bacteria by tagged sequencing : A comprehensive view in Enterococcus faecalis
Source: arXiv:1410.1925 ancillary file (2014-10-07)
Supplement: Supplementary file 1 [file MatSup.pdf]

# Supplementary Material

# Whole genome mapping of 5' RNA ends in bacteria by tagged sequencing: A comprehensive view in *Enterococcus faecalis*

Nicolas Innocenti[1,2,3], Monica Golumbeanu[4,5], Aymeric Fouquier d'Hérouel[1,6], Caroline Lacoux[2,3], Rémy A. Bonnin[7], Sean P. Kennedy[8], Françoise Wessner[2,3], Pascale Serror[2,3], Philippe Bouloc[7], Francis Repoila[2,3], and Erik Aurell[1,9]

October 7, 2014

**Short title :** Whole genome mapping of 5' RNA ends in bacteria

**E-mail :** njain@kth.se, monica.golumbeanu@bsse.ethz.ch, aymeric.dherouel@uni.lu, caroline.lacoux@jouy.inra.fr, remy.bonnin@u-psud.fr, sean.kennedy@jouy.inra.fr, francoise.wessner@jouy.inra.fr, pascale.serror@jouy.inra.fr, philippe.bouloc@u-psud.fr, **francis.repoila@jouy.inra.fr**, **eaurell@kth.se**.

* Co-corresponding authors.

**This file contains:**

**Section S1.** Design of the tags
**Section S2.** Raw sequencing output
**Section S3.** Prediction of transcription edges
**Section S4.** The 5' ends of Ref25C RNA
**Section S5.** Examples of known processing sites in *E. coli* retrieved by tagRNA-seq
**Section S6.** Long 3' untranslated regions
**Section S7.** Differential gene expression in static and respiratory growth
**Section S8.** Choice of the selection threshold for tag signals
**Section S9.** Accuracy of TSSs detection
**Section S10.** Description of the ppRNome Browser

## **Section S1.** Design of the tags

The SOLiD sequencing technology proceeds by shearing RNA molecules into small fragments and reading these in a massively parallel way [Metzker, 2010]. A typical RNAseq run results in several tens of millions of reads, each of 50 nt in length encoded in the SOLiD colorspace representation [Breu, 2010]. When using 5'tagRACE with PCR and gel electrophoresis-based methods, the length of the tags can be chosen to be around 30-40 nt to provide good specificity and stable binding of primers [Fouquier d'Hérouël et al., 2011]. However, when combining 5'tagRACE with RNA-seq on the SOLiD method, the use of such long tags is inappropriate due to the limited read length of this technology; such long tags would occupy most of the read leaving too little space for biological information to be of any use. We expect similar considerations to be relevant also for other sequencing platforms. Redesigning the tags to make them more suitable for tagged RNA-seq is thus a major step to make the whole procedure feasible. An important requirement for a good efficiency of tag ligation by the T4 RNA ligase is high purine content (75%) at their 3' end; we imposed the tags to end by GAA or AAA [Raabe et al., 2014, Wagner and Vogel, 2005].

The SOLiD colorspace encoding is designed in such a way that each sequence of 'colors' corresponds to four sequences of nucleotides [Breu, 2010]. Consequently, a candidate tag that appears to be specific in nucleotide representation may be mistaken for another sequence from the sample with the same colorspace representation. Thus the specificity of the tag with regard to the studied organism needs to be considered in the colorspace representation, i.e. the tag must be such that its colorspace representation is different from the colorspace representation of any subsequence of the genome. In addition, it is desirable for the tags to be as different as possible from each other to compensate for sequencing mistakes or other sources of errors, and minimise the risk of confusion.

Technically, a length constraint of the tags also applies due to the necessity to get rid of the excess (unligated to 5' RNA ends) after each RNA ligation step. Our methodology imposes a tag length $< 17$ nt to avoid affecting the total RNA content during the separation process. Finally, because of the limited read length of the sequencing technology, it is desirable for the tags to be as short as possible in order to have as much read length left for the biological information as possible. The final choice of tags is thus a tradeoff between the quantity of information in the biological sequence, technical constraints and the error tolerance of the tags.

We have set up a 3-step pipeline to generate suitable pairs of tags that takes as input the genome of a bacterium and a parameter E describing the desired error tolerance, and outputs a set of pairs of candidate tags. The first step in the procedure is to generate in a systematic way possible sequences. This is done by simple enumeration, from the shortest to the longest length considered. We then concatenate to each sequence the endings GAA and AAA and evaluate the purine content. Sequences that do not fulfil the requirement of purine content higher or equal to 75% are rejected. Secondly, for each candidate from the previous step, we then verify the specificity (in the colorspace representation) of the sequence itself as well as for all sequences that can be produced from the candidate by at most E substitutions, deletions or additions of nucleotides. A rigorous check of this kind would be computationally prohibitive. However, this step is very similar to another very common problem in the field of DNA/RNA sequencing: "the alignment", which, for a given reference sequence, consists in finding all the sequences in the genome that match the reference with at most E mismatches. Consequently, checking the specificity within an error tolerance of E is equivalent to failing at aligning the sequence to the genome with at most E errors. The alignment problem has been extensively studied for several decades and there are nowadays many efficient algorithms to perform this task [Klus et al., 2012, and references therein]. However, algorithms that are efficient enough

to be used in practice all rely on some sort of approximation that enables massive speed up in the search step. This means that any alignment software will, in some rare cases, miss some matches that should have been accepted within the provided error tolerance. Those misses are likely different for each software, but are deterministic for a given software running on a given genome. Therefore, we can turn the problem around by requiring that the same software is used for the design of the tags and for the alignments after sequencing. We can thus miss some possible tag pairs, but we will not mistakenly align a tag to the genome. In our case, the specificity and error tolerance steps were verified using Bowtie [Langmead et al., 2009], aligning in colorspace and the "-v" alignment mode allowing for E mismatches. Tags that fail to align are progressively added to two pools (ending in AAA and GAA) of good candidates. The procedure is stopped when a satisfactory number of good candidates have been discovered. Finally, the last step is to select, among the two pools of candidates available, the pairs that maximize the difference between the two tags. This step is achieved by performing a Smith-Waterman (SW) alignment [Smith and Waterman, 1981] between each pair of candidates and selecting the pair(s) that provide(s) the lowest alignment score. Although computationally inefficient, the SW alignment is applied to a not too numerous set of candidates of modest length and is thus computationally feasible. In the present case, the pair TSS-tag (5'-GCGAGACUGAGAA-3') and PSS-tag (5'-GCAUAGGGGUAAA-3') were obtained by applying the procedure described above using the genome of *E. faecalis* V583 (reference sequences with NCBI accession numbers [GenBank:AE016830] to [GenBank:AE016833]). The numbers of sequences with lengths 11, 12 or 13 nt for error tolerance of 0, 1 or 2 are shown in figure S1. We note that no sequences shorter than 11 nt satisfying the specifications were found. 4 sequences of 13 nt long ending in GAA were found to satisfy the specificity with 'E = 2', but no such sequences were found with AAA ending. We decided to restrict the tags to a length of 13 nt and focus on the 4 candidates with error tolerance E = 2. Out of the roughly 20 000 sequences in the AAA-end pool with E = 1, the Smith-Waterman alignment gave between 6 and 50 equally good partner sequences. TSS-tag and PSS-tag use in this study were arbitrarily chosen among this set of sequences.

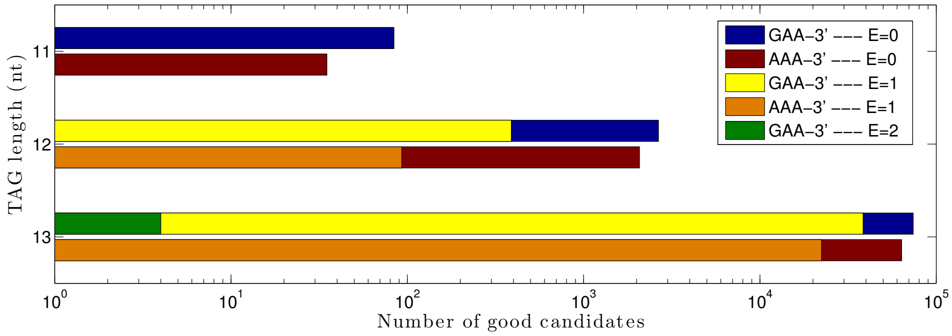


**Figure S1:** Number of tags of 11, 12 and 13 nt long with different error tolerances.

As for *E. coli*, because of the larger genome with a more neutral GC-content in comparison to *E. faecalis*, a comparable error tolerance of 2 requires longer sequences. Nevertheless, we verified that the tags as designed for *E. faecalis* are also absent from the *E. coli* U00096.3 and used them as well for tagging *E. coli* RNA in order to facilitate several experimental steps. Given the observed high accuracy of RNA-seq on the tag sequences (**Section S2.**) and provided the lower error tolerance is taken into account in the analysis, the impact of such a choice is negligible.

## Section S2. Raw sequencing output

Global results from RNA-seq experiments are summarised in table S1 for *E. faecalis* and in table S2 for *E. coli.* A description of the samples and their preparation can be found in Materials and Methods.

### SOLiD 3 RNA libraries

| | rRNAs present "KTH" transcriptome | | rRNAs removed "KTHr" transcriptome | |
|---|---|---|---|---|
| | **Reads** | **% of total (previous)** | **Reads** | **% of total (previous)** |
| **Total** | 120 572 828 | 100% | 125 763 371 | 100% |
| **Mapped** | 49 294 643 | 40.8% | 41 776 633 | 33.2% |
| **Mapped in rRNA** | 42 828 356 | 35.5% (86.9%) | 13 099 245 | 10.4% (31.4%) |

### Illumina RNA library

| | "IlluminaSt" transcriptome | |
|---|---|---|
| | **Reads** | **% of total (previous)** |
| **Total** | 56 425 007 | |
| **Remaining after adapter removal** | 44 158 978 | 78.2% |
| **Mapped** | 39 032 892 | 69.2% (88.4%) |
| **Mapped in rRNA** | 37 987 679 | 67.3% (97.3%) |

### SOLiD 5500 tagged RNA libraries

| | "Rt" transcriptome | | "St" transcriptome | |
|---|---|---|---|---|
| | **Reads** | **% of total (previous)** | **Reads** | **% of total (previous)** |
| **Total** | 71 287 382 | | 66 627 584 | |
| **Without tags** | 65 291 792 | 91.6% | 62 636 046 | 94.0% |
| **Mapped** | 34 048 489 | 47.8% (52.1%) | 33 984 161 | 51.0% (54.3%) |
| **Mapped in rRNA** | 31 625 325 | 44.4% (92.9%) | 32 129 015 | 48.2% (94.5%) |
| **With TSS-tag** | 2 206 697 | 3.1% | 1 419 828 | 2.1% |
| **No error in tag** | 1 678 955 | 2.4% (76.1%) | 1 085 208 | 1.6% (76.4%) |
| **Mapped** | 829 521 | 1.2% (37.6%) | 561 621 | 0.8% (39.6%) |
| **Mapped in rRNA** | 218 231 | 0.3% (26.3%) | 183 792 | 0.3% (32.7%) |
| **With PSS-tag** | 3 340 293 | 4.7% | 2 172 190 | 3.2% |
| **No error in tag** | 2 392 558 | 3.4% (71.6%) | 1 652 182 | 2.5% (76.0%) |
| **Mapped** | 1 595 507 | 2.2% (47.8%) | 1 170 366 | 1.8% (53.9%) |
| **Mapped in rRNA** | 920 665 | 1.3% (57.7%) | 679 731 | 1.9% (58.1%) |

**Table S1:** Summary of raw sequencing results in *E. faecalis.*

Quantitative data analysis of the "St" and "Rt" transcriptomes discussed in extensive details in the paper yielded 66.6 and 71.3 millions of total reads, respectively. Out of those, and permitting at most two sequencing errors in the tag, we were able to map for Rt and St: i) 52.8% and 54.7% of reads with no tags; ii) 28.6% and 28.7% of reads with TSS-tags, representing 3.8% and 2.8% of total reads, respectively, and iii) 35.5% and 41% of reads with PSS-tags,

**SOLiD Wildfire tagged RNA library**

| | "Coli" transcriptome | |
|---|---|---|
| | **Reads** | **% of total (previous)** |
| **Total** | 136 574 252 | |
| **Remaining after adapter removal** | 97 166 615 | 71.2% |
| **Without tags** | 89 553 433 | 65.6% (92.2%) |
| **Mapped** | 26 960 785 | 19.7% (30.1%) |
| **Mapped in rRNA** | 23 557 114 | 17.3% (87.4%) |
| **With TSS-tag** | 2 705 707 | 1.98% (2.78%) |
| **Mapped** | 530 719 | 0.39% (19.6%) |
| **Mapped in rRNA** | 145 134 | 0.11% (27.3%) |
| **With PSS-tag** | 1 658 796 | 1.71% |
| **Mapped** | 600 184 | 0.44% (36.2%) |
| **Mapped in rRNA** | 341 584 | 0.25% (56.9%) |

**Table S2:** Summary of raw sequencing results in *E. coli.*

corresponding to 5.4% and 3.8% of total reads, respectively. Those numbers confirm that samples were of similar quality and the sequencing procedure worked in a similar manner in both cases.

Interestingly, while almost 90% of untagged reads fall into rRNA regions, the proportion is much smaller for reads carrying TSS- and PSS-tags, about one third and two thirds respectively.

In order to account for variations in total number of reads and be able to compare experiments, RNA levels are reported normalised to the total number of reads mapped, as it is commonly done in RNAseq. Additionally the ligation procedure introduces a new variability in the experiment that is average out by normalising the number of tagged reads mapped at a given position to the total number of tagged reads mapped for the entire V583 genome (Table SA).

The comparison between the annotated genome of V583 *E. faecalis*, and St and Rt indicate that out of the 3.34 Mbp long genome, respectively 1.5 and 1.8 Mbp appears to be transcribed (coverage higher than 2x), respectively. These transcribed regions encompass 49% to 58% of the annotated sequences (i.e. ORFs, r- and tRNAs that represent 2.88 Mbp of the total genome), 2 (~73 kb) to 3% (111 kb ) being due to antisense transcription, and 29% to 36% of non-annotated and/or non-coding portions (i.e. 5'- and 3' UTRs, unannotated ORFs, and as- and sRNAs, 0.47 Mbp). On the other hand, ~1.3 and 1.1 Mbp appears without any signal (coverage equal zero), representing ~30% of annotated regions and ~55% to 60% of non-annotated ones, in St and Rt, respectively.

Two untagged libraries obtained from S growth conditions were sequenced on the (older) SOLiD 3 platform. In these libraries rRNAs were removed or conserved, providing transcriptomes "KTHr" and "KTH", respectively.

Table S3 shows that the mapping rates observed in those transcriptomes can be raised arbitrarily high by filtering out reads of low quality. This indicates that the lower mapping rate observed compared to other platforms are only due to somewhat lower quality reads from the SOLiD 3 (a contamination from foreign RNA would cause a constant fraction of unmappable reads even for reads with very high quality). Given the large gap between the SOLiD 3 and 5500 platforms, such improvements in overall quality are not out of lines of expectations.

Furthermore, a more detailed analysis of the table allows to conclude that i) the platform produces virtually no reads with qualities in the 0-10 range and ii) the removal of the rRNA does affect other RNAs in some unknown manner (at least in our experiment) as the mappable fraction remains lower even for high quality reads.

In the IlluminaSt dataset, a fraction of reads (∼21%) are discarded during the adapter removal process due to the very short (¡18 nt) bacterial RNA fragments they carry. The mapping rate for the remaining ones is the highest observed among our different transcriptomes. While this library yielded a similar number of mapped reads compared to the four other transcriptomes, the average read length after adapter removal is shorter than 50nt and thus the total coverage is lower.

| Read quality threshold | Rejected fraction | | Mapped fraction (mapped reads) | |
|---|---|---|---|---|
| | KTH | KTHr | KTH | KTHr |
| 0 | 8.8% | 8.7% | 42.46% (46.7 Mreads) | 34.45% (39.6 Mreads) |
| 5 | 8.8% | 8.7% | 42.46% (46.7 Mreads) | 34.45% (39.6 Mreads) |
| 10 | 11.1% | 10.5% | 43.43% (46.5 Mreads) | 35.02% (39.4 Mreads) |
| 15 | 31.3% | 27.7% | 54.53% (45.2 Mreads) | 41.99% (38.2 Mreads) |
| 20 | 55.7% | 52.5% | 73.97% (39.5 Mreads) | 56.34% (33.7 Mreads) |
| 25 | 81.1% | 78.5% | 89.21% (20.3 Mreads) | 71.70% (19.4 Mreads) |
| 30 | 99.1% | 99.46% | 97.17% (0.97 Mreads) | 85.59% (0.58 Mreads) |

**Table S3:** Filtering out reads with low quality arbitrarily improves the mapping rate in the KTH sample at the cost of discarding a fraction of mappable reads. The quality of a read is defined as the average quality of each of its letters. The column "Read quality threshold" shows the threshold below which a read is rejected. A read quality threshold of 0 means that only reads with uncalled bases are removed.

The "Coli" transcriptome was sequenced on a newly installed SOLiD Wildfire platform at (MetaGenomPolis, INRA, France). Compared to the SOLiD 5500, this platform at its current stage of development is known to produce a higher number of raw reads with an overall lower quality, leading to a roughly similar number of usable reads, as observed by comparing the tables.

## Section S3. Prediction of transcription edges

The principle of the edge detection algorithm described in "Materials and Methods" of the article, is illustrated in figure S2. The algorithm was used with a confidence threshold set to 5 unique reads. Visual inspection of the data in GBrowse (see below) suggests that this configuration provides good sensitivity and reliable predictions for regions with sufficient expression level, where the coverage depth signal is continuous, but generates many predictions that we believe to be false positives in lowly expressed regions, where the coverage becomes discrete. We note that an approach based on a hidden markov model (HMM), documented elsewhere [Golumbeanu, 2013], to perform the same predictions on the same data showed slightly improved specificity at the cost of much higher computational load.

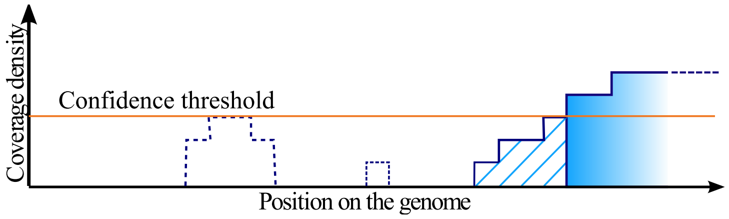


**Figure S2:** Proposed edge detection algorithm. For each signal above a chosen threshold is marked as strong signal (blue region). Low signal is iteratively annexed to the strong signal region (blue-hatched region). All signal that was not marked as strong at the end of the procedure is disregarded (dashed line).

We ran the edge detection algorithm on the RNA-seq data obtained with tagged and untagged total RNA extracted from cells grown in S conditions ("St" and "KTH" transcriptomes). The results were compared and we observed that 5' edges in both transcriptomes are found at similar location (less than 4 nt apart), indicating that the addition of tags does not affect the location of edges of transcribed regions (Figure S3).

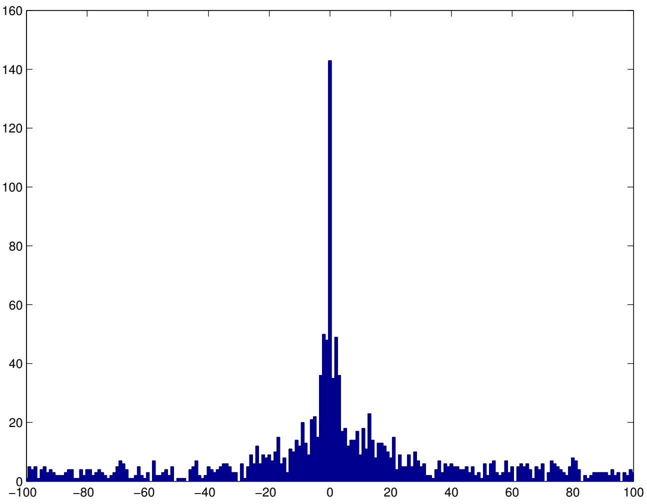


**Figure S3:** Histogram of the distances between edges predicted in the tagged (St) and untagged (KTH) experiments. .

Combining predictions from the algorithm and signals provided by tags enable us to sort

potential TSSs that match with the intuitive idea of a TSS, i.e. the absence of detectable expression level upstream and clear expression level downstream (example in figure S4A), from other less obvious situations (example in figure S4B). A global comparison between predictions and tag counts was performed to obtain the figure "below 30°" in the main manuscript (Figure 2A), where we kept only points in the cloud that are within 4 nt of a predicted rising edge along the same strand.

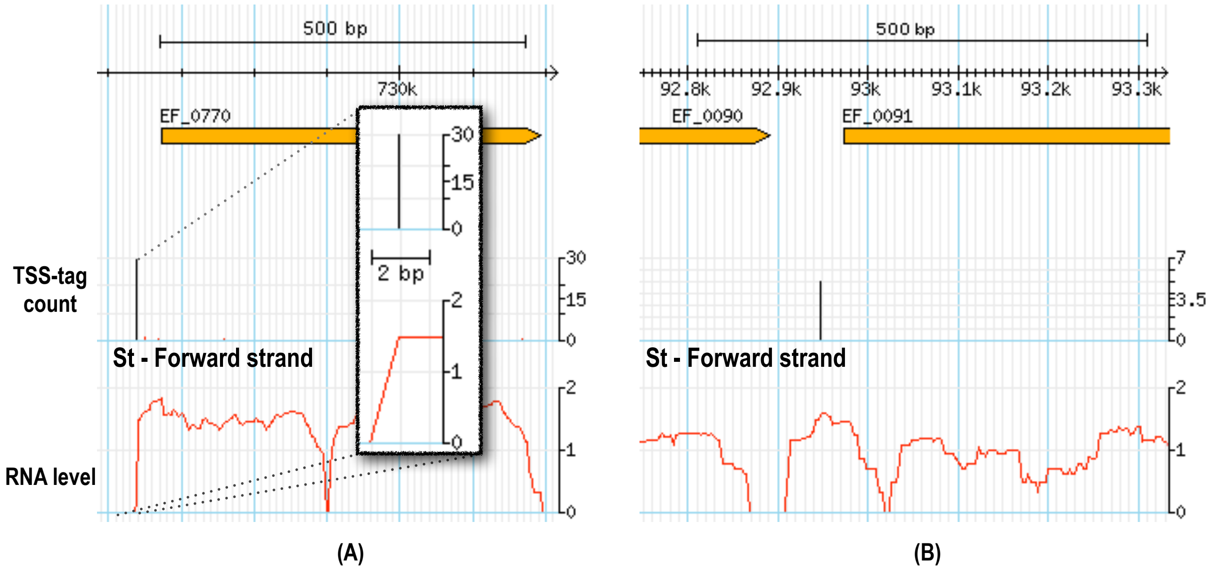


**Figure S4:** (A) Example of a TSS-tag signal matching with the intuitive idea of a TSS, i.e. the absence of detectable expression level upstream from the tag location and clear expression level downstream. (B) Example of a TSS-tag signal at position 92950 nested in a longer transcribed region and not matching with intuition.

## Section S4. The 5' ends of Ref25C RNA

The transcript expressed from gene *ref25C* was previously characterised and the TSSs was mapped at position 569154 [Fouquier d'Hérouël et al., 2011]. In agreement with these results, tagRNA-seq mapping allocates as TSS three nucleotides for Ref25C, 569154, 569155 and 569156 (Table SA). Based on the position 569154 and on the 3' end mapping of the RNA, we showed that Ref25C RNA can be overexpressed with an identical length as the transcript expressed from the chromosome when the gene was cloned on a multicopy plasmid (225 bp), attesting that the promoter region deduced from the RNA mapping was contained in the cloning vector (see Figure S5 in [Fouquier d'Hérouël et al., 2011]). Furthermore, a transcriptional fusion encompassing only 305 bp upstream from the TSS mapped (coordinate 569154) is sufficient to drive the transcription of the *lacZ* encoding sequence used as reporter system in *E. faecalis.* For comparison, the plasmid vector (p-lacZ, a derivative vector of pVE14189, [Dumoulin et al., 2013]) and DNA portions of 455 bp and 56 bp nested in 16S and 23S rRNAs encoding sequences, respectively, were not active as measured in $\beta$-galactosidase assays (not shown) or visualized on BHI plates containing 5-bromo-4-chloro-3-indolyl-beta-D-galactopyranoside (X-Gal), (Figure S5; C. Lacoux and F. Repoila, *unp. data*). The promoter of the *fsrA* gene ($P_{fsrA}$) was used as positive control [Qin et al., 2001]. These data indicate that the upstream region from the TSS mapped at positions 569154/-56 by tagRNA-seq contains an active promoter. This conclusion is reinforced by i) no significant RNA levels were detected within the 300 bp upstream from tags detected (see browser and table SA), ii) -10 (TATAAT) and -35 (TTGAGC) hexamers highly similar to canonical promoter sequences, and spaced by 17 bp are found upstream from the mapped positions 569154/-56. Although the upstream-most 5' end mapped for Ref25C RNA appears above the diagonal figure 2B, experimental data here above indicate that this 5' RNA end is a true TSS.

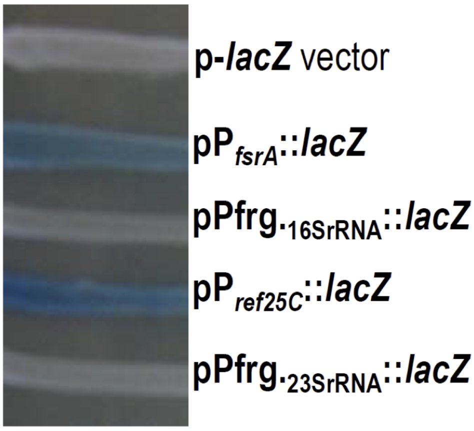


**Figure S5:** $\beta$-galactosidase activities observed on BHI plates containing X-gal. The following DNA fragments were used to drive the *lacZ* transcriptional fusion in a pVE14189 derivative plasmid [Dumoulin et al., 2013]: p-*lacZ* vector empty; p$P_{ref25C}$*::lacZ*, *lacZ* encoding sequence fused to 305 bp upstream of the TSS mapped for *ref25C* (coordinate 569154, Tables SA); p$Pfrg_{16SrRNA}$*::lacZ*, 455 bp nested in 16S rRNA; p$Pfrg_{23SrRNA}$*::lacZ*, 56 bp nested in 23S rRNA; p*PfsrA::lacZ*, *lacZ* encoding sequence fused downstream the *fsrA* promoter used as positive control [Qin et al., 2001]. The strain VE18581 containing the construct p*PfsrA::lacZ* was kindly provided by Stéphane Gaubert.

## Section S5. Examples of known processing sites in *E. coli* retrieved by tagRNA-seq

Examples of processing sites in *E. coli* reported in the literature retrieved by tagRNA-seq together with tag signals retrieved by tagRNAseq are presented in table S4. In this table, we also include cases that are called as undetermined or that falls below the selection threshold in our experiment.

| **Previously reported PSS** | | | | **tagRNA-seq result** | | |
|---|---|---|---|---|---|---|
| **Position** | **Strand** | **Region** | **Ref.** | **Position** | **Tag count** | **Angle** |
| 20910 | - | rpsT | (A) | 20908/-10 | 31 | 36° |
| 21021 | - | rpsT | (A) | 21018 | 2 | 90° |
| 2755593 | + | ssrA | (B) | 2755593 | 117 | 75° |
| 3055983 | | ssrS | (C) | 3055983 | 660 | 90 ° |
| 3212852 | + | dnaG-rpoD | (D) | 3212852/-3 | 6 | 45 ° |
| 3270495 | - | rnpB | (E) | 3270495 | 3 | 63 ° |
| 3913829 | - | glmU-glmS | (F) | 3913827 | 4 | 72 ° |
| 3982501 | + | argX-hisR | (G) | 3982501 | 8 | 59° |
| 3982586 | + | hisR-leuT | (G) | 3982586/-9 | 34 | 80 ° |
| 3982705 | + | leutT-proM | (G) | 3982705 | 41 | 84 ° |
| 3982731 | + | leutT-proM | (G) | 3982731 | 5 | 76 ° |
| 4035465 | + | rrsA | (H) | 4035465 | 238 | 67 ° |
| 4035530 | + | rrsA | (H) | 4035528/-31 | 9943 | 77 ° |
| 4037073 | + | rrsA | (H) | 4037073 | 2155 | 90 ° |
| 4037106 | + | rrsA | (H) | 4037106 | 171 | 56 ° |
| 4040442 | + | rrlA-rrfA | (I) | 4040442 | 105 | 56 ° |
| *Indirect evidence*(1) | - | yfiD | (K) | 2716466/-76 | 10 | 90 ° |
| *Indirect evidence*(2) | - | rpsU | (K) | 3210759 | 23 | 87 ° |

**Table S4:** Examples of processing sites known in *E. coli* retrieved by tagRNA-seq and tag signals at the corresponding positions. The coordinates given correspond to the first nucleotide after each cleavage site. The tag count columns gives the raw tagged read count (TSS+PSS).

(1) : Figure 1 (A) in [Vesper et al., 2011] clearly shows one or more non MazF-dependent cleavage sites about 20 bp upstream of the reported mazF "A" site (271651). In the present case, multiple PSS-tags are observed in the AT-rich corresponding region, suggesting RNAse E activity.

(2) : Figure S1 (B) in supplementary material of [Vesper et al., 2011] shows two non mazF-dependent cleavage sites around respectively 10 and 20 bp upstream of the reported mazF "A" site (3210779). The latter region is AT-rich and contains clear tag signals indicating a PSS.

References in the table : (A) : [Mackie, 2013] ; (B) : [Lin-Chao et al., 1999] ; (C) : [Kim et al., 2004] ; (D) : [Yajnik and Godson, 1993] ; (E) : [Lundberg and Altman, 1995] ; (F) :[Urban and Vogel, 2008] ; (G) : [Kime et al., 2014] ; (H) : [Li et al., 1999] ; (I) : [Gutgsell and Jain, 2012] ; (K) : [Vesper et al., 2011].

## Section S6. Long 3' untranslated regions

Using the edge detection algorithm described in section **Section S3.**, we predicted the 3'end of transcripts corresponding to annotated ORFs with the additional constraint that the coverage has to remain zero for at least 40 bp downstream of a predicted end. We also restricted our search to transcribed annotated ORFs having a non-zero coverage over at least 75% of their length, and considered only the last ORF of an operonic organization when such a situation applied. We measured the length of the 3'UTR as the distance between the predicted 3'end of the transcript and the last nucleotide of the translation stop codon of the corresponding annotated ORF; the distributions of those lengths for Rt and St are shown in figure S6.

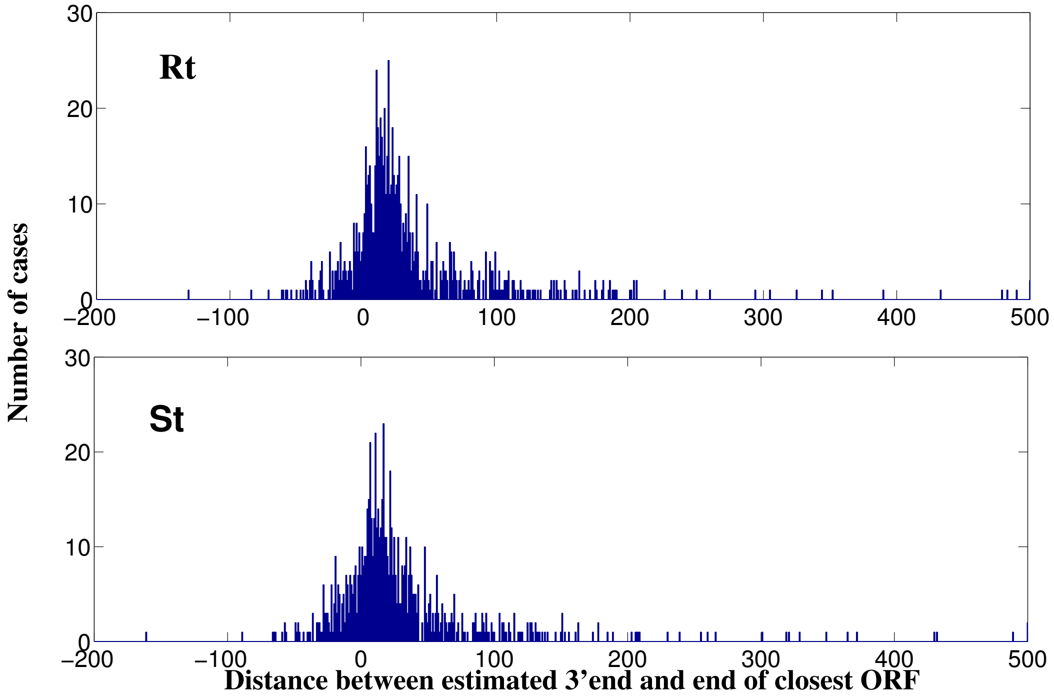


**Figure S6:** (Distribution of the 3'UTRs estimated lengths for annotated ORFs in Rt (top) and St (bottom). Two cases for which the estimated 3'UTR length was greater than 500 nt fall outside of the region shown above.

For each transcriptome, distributions are centered between 0 and 100 bp downstream from the ORFs indicating that most of 3' UTRs appear short (≤100 nt). On the contrary, a few 3'UTRs were found with a length >200 nt and were further manually screened based on the quality of the RNA signal. Table S5 presents the selected list of long 3' UTRs found in the V583 genome.

We analysed tagRNA-seq data in order to reveal the extension of transcripts downstream annotated ORFs and detect long 3' UTRs (Section S5). The sequencing method used in our experiments is known to underestimate the length of the 3'UTRs [Innocenti and Aurell, 2013]. Consequently, transcripts displaying apparent 3' UTRs longer than 200 nt can be safely considered as long 3'UTRs. We analysed the latter and eliminated those for which TSSs were nested in the end of corresponding ORFs or within 3' UTRs, and those presenting a low coverage signal (Section S5). We found 19 ORFs carrying long 3' UTRs ranging from ∼200 nt to ∼560 nt,

including 6 of them that form antisense organisations with flanking ORFs transcribed from the complementary DNA strand (Table S2). In contrast to eukaryotes where the fate of an mRNA is mainly dependent on numerous *trans*-factors binding to the 3'UTR [Brodersen and Voinnet, 2009, Garneau et al., 2007, Matoulkova et al., 2012], in bacteria, the significance of long 3' UTRs is poorly understood. A series of experiments have shown that some of them are preferentially bound by the chaperon RNA protein Hfq in *S. typhimurium* [Chao et al., 2012, Sittka et al., 2008] and the RNase III in *S. aureus* [Lioliou et al., 2012], indicating the interaction of 3' UTRs with major factors involved in RNA-mediated regulation. For example, in *S. aureus* the long 3'UTR of *icaR* mRNA, that encodes a major transcription regulator involved in virulence and biofilm development, pairs to the 5'UTR of *icaR* mRNA via an intra- and/or inter-molecular mechanism, represses translation and destabilises the transcript [Ruiz de los Mozos et al., 2013]. Long 3' UTRs have been reported in several species across the bacterial kingdom suggesting that these RNA elements can be sources of genetic information and regulatory processes that require further investigation [Chao et al., 2012, Nicolas et al., 2012, Rasmussen et al., 2009, Ruiz de los Mozos et al., 2013, Sittka et al., 2008, Toledo-Arana et al., 2009].

| ORF | 3'UTR length $\geq$ 200 nt | Comments |
|---|---|---|
| EF_0052 | 322 | antisense to 3' end of EF_0051 |
| EF_0157 | 352 | |
| EF_0405 | 305 | antisense to 3' end of EF_0404 |
| EF_0478 | 423 | antisense to near the entire ORF EF_0479 barely expressed |
| EF_0521 | 203 | |
| EF_0566 | 296 | |
| EF_0571 | 200 | |
| EF_0610 | 490 | |
| EF_0747 | 479 | |
| EF_1097 | 260 | |
| EF_1114 | 250 | |
| EF_2022 | 559 | |
| EF_2282 | 226 | antisense to EF_2283 as predicted by transcription terminators |
| EF_2512 | 205 | |
| EF_2518 | 344 | |
| EF_2643 | 201 | |
| EF_2995 | 390 | antisense to EF_2996 that is not expressed |
| EF_3207 | 203 | antisense to a stand-alone sRNA whose TSS is not detected by tags |
| EF_3278 | 544 | |

**Table S5:** Long 3' UTRs detected in the St and Rt. Candidates (Figure S6) that were detected due to weak signal in the tail or obvious sequencing artefacts have been removed.

## **Section S7.** Differential gene expression in static and respiratory growth

As an additional verification step of our samples, we performed a differential expression analysis using "Cuffdiff" from the Cufflinks suite[Trapnell et al., 2010] (Materials and Methods). The list of ORFs that displayed significant variation of RNA levels between the two conditions is available in Table SD.

Cufflinks calls a significant variation based on a probabilistic model such that when the number of replicates is low a conservative estimate is made, and the false negative rate using only one data set for each condition can therefore be expected to be large [Trapnell et al., 2010]. Comparing Rt and St, we obtained a list of 31 ORFs that displayed significant variation of RNA levels between the two tagged RNA-seq. We assessed the false positive rate by comparing to the results including in the analysis data from the "IlluminaSt" transcriptome in the S growth condition. This improves the prediction quality of some called genes (decreases p-values for 16 ORFs), adds 16 more called genes to the list (moves their p-values below threshold), and still calls 23 ORFs in the list. For the nine ORFs that are removed from the list, the p-value, on the other hand, increases above threshold.

Annotation and gene ontology information show that most of the genes in this list are involved in the central metabolism associated with the consumption of sugars and amino acids as carbon and nitrogen sources, mainly centered on glycolysis, pyruvate metabolism and citrate cycle (TCA) (`http://www.genome.jp/kegg/pathway.html` and Figure S7). For instance, operons *celAB*, *ef1017-ef1020* and *ef2959-ef2961* have a higher expression in S compared to R conditions, and are predicted to code for phosphor-sugar transfer systems (PTSs) of cellobiose and ribose uptake, and degrading enzymes, respectively. These transporter systems allow the entry and the phosphorylation of specific sugars that are catabolized via the glycolytic pathway. In R, compared to S conditions, an increased expression is detected for operons *ef0097-ef0100* that code for the subunits of the serine-dehydratase (Sdh) that converts serine into pyruvate (or the reverse reaction), the end product of glycolysis, and *ef1657-ef1663* coding for enzymes that feed or make part of the TCA cycle and glycolysis, and participate to amino acid metabolism (valine and serine) from pyruvate. An increased expression in R conditions was also observed for operon *glpFOK* (*ef1927-ef1929*) coding for enzymes enabling glycerol catabolism via glycolysis in aerobic conditions [Bizzini et al., 2010].

The results of this standard differential expression analysis are in line with previous reports on metabolic and transcriptomic studies performed on *E. faecalis* and closely related species such as *L. lactis* [Cocaign-Bousquet et al., 1996, Garrigues et al., 1997, Pedersen et al., 2008b]. Under S conditions (anaerobic growth) and in the growth medium used in this study *E. faecalis* adopts fermentation, a physiological state characterized by a high rate of sugar consumption in comparison to respiration, and employs the glycolysis pathway for glucose catabolism, ending up in pyruvate formation [Garrigues et al., 1997, Pfeiffer et al., 2001]. In *E. faecalis*, the respiratory chain is complete but not functional as genes encoding enzymes required for heme synthesis are absent. However, if oxygen and heme are supplied, as in R growth conditions, *E. faecalis* switches from homolactic fermentation to respiration and under respiration, pyruvate conversion is not exclusively catalyzed by Ldh-1, but also by Als (Ef1213), Pdh (Ef1353/Ef1354), Pfl (Ef1612/Ef1613) and AdhE (Ef0900), ending in the production of various products (acetate, ethanol, formate), and regenerate NAD+ from NADH [Pedersen et al., 2008a, Winstedt et al., 2000, Yamamoto et al., 2006].

In summary, with the caveats of high expected false negative rate when comparing few samples, it can be checked that all the reported variations in Figure S7 and Table SD are consistent with previously reported features of *E. faecalis* biology with and without respiration.

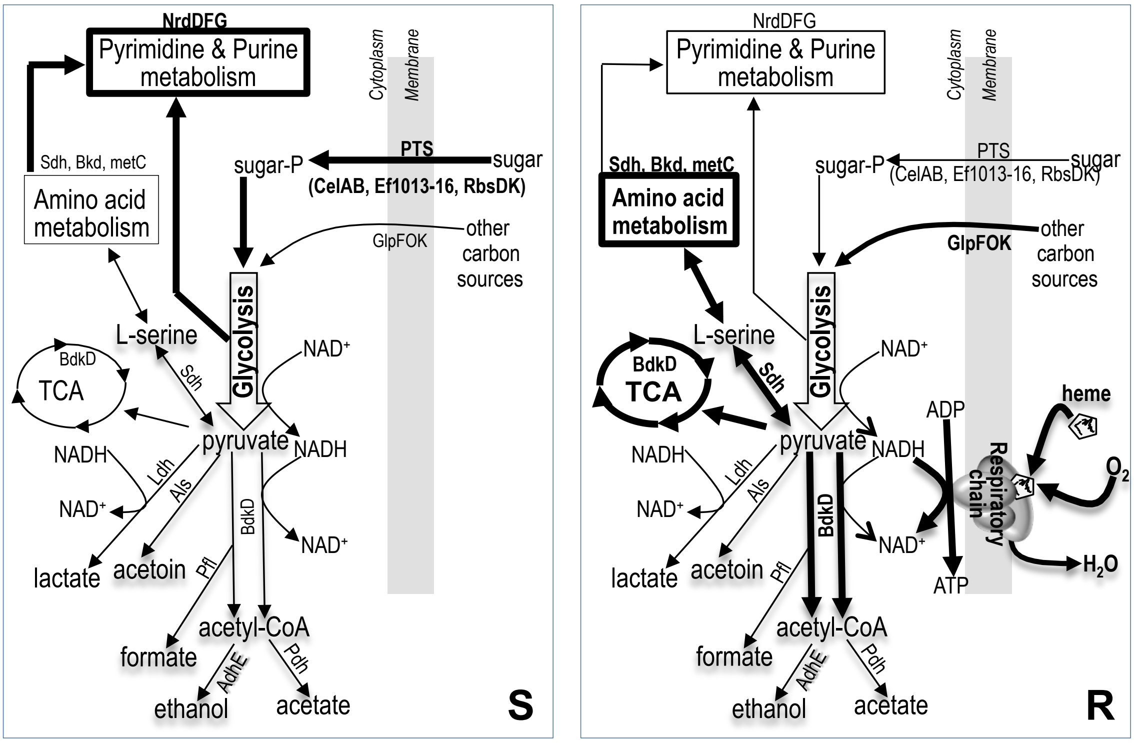


**Figure S7: Metabolic pathways deduced from functions assigned to RNAs differentially expressed in S and R growth conditions.** Transcriptomes St and Rt both show significant expression of genes involved in central metabolism, but assuming that mRNAs detected are translated into proteins and that these proteins are active, differential expression analysis indicates that groups of enzymes specifically involved in certain pathways of the central carbon metabolism are induced. In static growth conditions (S), sugar uptake systems (PTSs) and nucleotide bases metabolism; pathways and gene products induced are shown with dash arrows and in grey. In respiration (R), the formation of acetyl-CoA from pyruvate, formate and ethanol are enhanced, as well as the citrate cycle (TCA) and amino-acids metabolism; pathways and gene products induced are shown with thick arrows and bold characters. Major enzymes involved are indicated. Their names are indicated in tables SD and assigned functions are those reported in the KEGG website database.

## **Section S8.** Choice of the selection threshold for tag signals

Figure S8 shows the distribution of the number of genomic locations with a tag signal greater or equal to a threshold as a function of that threshold for the three tagRNA-seq experiments presented in this work. Above two or three reads, the resulting curves behave as power laws, demonstrating that no "natural threshold" is present in the data. The "Coli" transcriptome behaves in a similar way to the "Rt" and "St", except for an overal lower level of signal due to a slightly smaller number of reads spread over a 40% larger genome. Varying the threshold simply changes the number of accepted candidates.

The values of roughly 5 reads chosen in this work are a reasonable choice that eliminates the latter while maintaining a fair sensitivity for the detection.

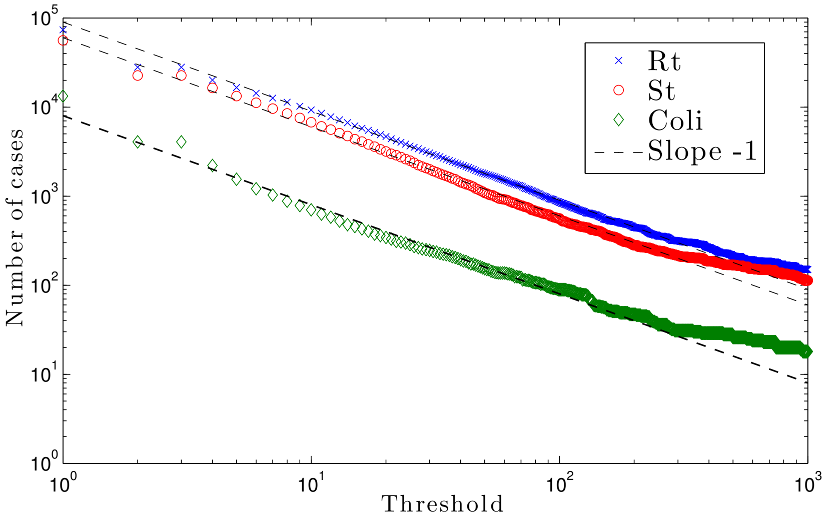


**Figure S8:** Number of positions where the raw tag signal (TSS+PSS) is greater than or equal to a threshold as a function of this threshold for the Rt, St and Coli transcriptomes. The dashed black lines plotted near the data points show power laws with exponent $-1$.

## **Section S9.** Accuracy of TSSs detection

As mentioned in section *"Detection of transcription starts and processing sites using 5' tags"*, transcription at a transcription start site is not always initiated with single nucleotide accuracy [Cortes et al., 2014, Morton et al., 2014, Schluter et al., 2013, Sharma et al., 2010] and our detection scheme takes this into account by grouping tag signals distant by 4 nt or less from each other when at least one of them is classified as a TSS candidate.

As a result, a TSS as reported in Table SC is not a single point location, but a region with a start, an end and a width. The distribution of the widths of reported TSSs is shown in figures S9(a) for *E. faecalis* and (b) for *E. coli.* Almost all TSSs reported are mapped with an accuracy of 6 nt or less, and a large fraction of them with single nucleotide resolution.

Furthermore, we have studied in Figure S9(c) the distribution of tag signal (TSS+PSS) around reported TSSs. The figure shows that most of the signal concentrates in the region ± 2 bp around the reported locations as given in Table SC.

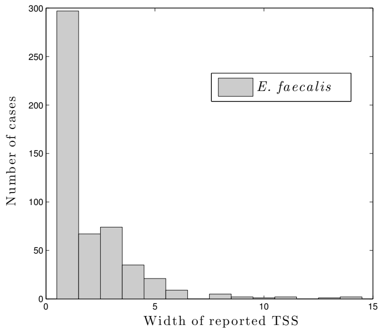


(a)

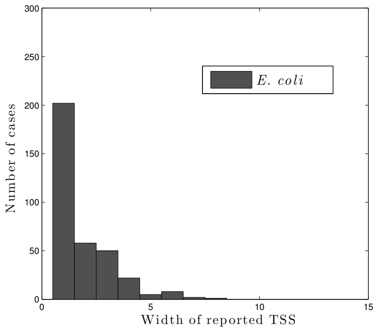


(b)

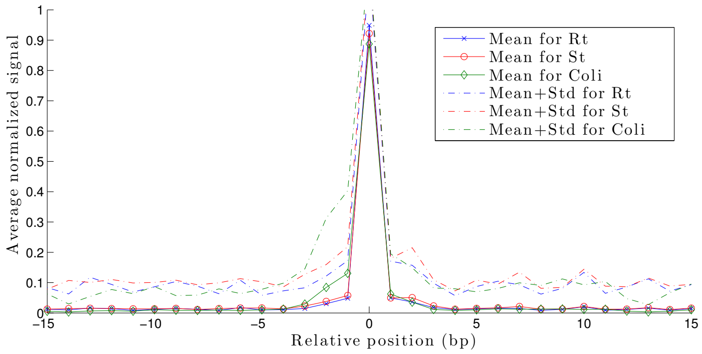


(c)

**Figure S9:** (a) Distribution of the widths of TSSs retrieved by tagRNA-seq in *E. Faecalis v583.* (b) The same in *E. Coli* K12 MG1655. (c) Average normalised signal around the most probable position of each TSSs retrieved for the St, Rt and Coli transcriptomes. The signal around each TSS is normalised so that its maximum value on the range considered is 1. The dashed lines represent one standard deviation from the average normalised signal in order to get an estimate of the variability of the signals.

## **Section S10.** Description of the ppRNome Browser

A user-friendly visualization of all the data introduced in this work, called ”the ppRNome Browser”, is available online at the address `http://ebio.u-psud.fr/eBIO_BDD.php` (select database named “ppRNome”) using the Generic Genome Browser (GBrowse), an open-source software developed within the Generic Model Organism Database project ([Stein et al., 2002] and GMOD homepage[1]). The data presented in the browser is also available in a numerical format in Table SA (significant tag signals) and Table SB (gene expression level) for the Rt and St transcriptomes.

The main page of GBrowse starts with several tabs at the top, the two most important of which being ”Browser” - the one selected by default when loading the page - and ”Select Tracks” - the one allowing to select which data to display.

In the ”Browser” tab, a search box allows to navigate directly to genomic loci using the annotation (e.g. “EF_1980”, “EF_23S”,) or directly by coordinates (e.g. “AE016830:250246..253154”). The ”Data Source” menu allows to select the chromosome or one of the two plasmids of *E. faecalis* strain VE14002 (V583 derivative) or the chromosome of *E. Coli* K12 sub-strain MG1655.

Once a data source is selected, the ”Overview”, ”Region” and ”Details” bar allow to navigate interactively along the selected chromosome or plasmid with variable accuracy. Under the navigation bars come the data tracks that show different kinds of information. By default, for *E. faecalis* the browser will display only 3 data tracks showing, from top to bottom, the coverage signal on the forward strand for the untagged RNA-seq in S growth conditions with rRNAs, the genomic annotation obtained from NCBI and the coverage signal on the reverse strand from the same data set. For *E. coli*, the coverage signal tracks are those from the ”Coli” transcriptome. The user can modify the order of the tracks by simple drag and drop on the title bar of the track. Color, scale and other parameters used to display the data on the track can be modified by clicking on the icon showing a wrench in the corresponding title bar (for documentation on the different options available, see the user manual on GBrowse’s homepage).

The ”Select Tracks” tab on top of the page allows selecting more data tracks to be shown in the browser. Selectable tracks contain general genomic annotations (NCBI annotation, GC content, start/stop codons, rho-independent terminators,...) and all the data from our experiments (coverage signal and tag signals on each strand for the different transcriptomes available). In addition, for *E. faecalis*, we created a few special tracks combining two or more of the previously described ones, which, while they do not bring any new information, help to compare results across the different experiments. Below the list of available tracks, a legend describes for each group of data tracks the type of data shown as well as the scaling and/or normalisation used. The user can select and display as many tracks as desired simultaneously. However, a large number of tracks can significantly slow down the interactive navigation.

[1] `http://www.gmod.org`

## References


A. Bizzini, C. Zhao, A. Budin-Verneuil, N. Sauvageot, J. C. Giard, Y. Auffray, and A. Hartke. Glycerol is metabolized in a complex and strain-dependent manner in Enterococcus faecalis. *J Bacteriol*, 192(3):779–85, 2010. ISSN 1098-5530 (Electronic) 0021-9193 (Linking). doi: 10.1128/JB.00959-09.

Heinz Breu. A Theoretical Understanding of 2 Base Color Codes and Its Application to Annotation, Error Detection, and Error Correction. Applied Biosystems, 7 2010.

P. Brodersen and O. Voinnet. Revisiting the principles of microRNA target recognition and mode of action. *Nat Rev Mol Cell Biol*, 10(2):141–8, 2009. ISSN 1471-0080 (Electronic) 1471-0072 (Linking). doi: 10.1038/nrm2619.

Y. Chao, K. Papenfort, R. Reinhardt, C. M. Sharma, and J. Vogel. An atlas of Hfq-bound transcripts reveals 3' UTRs as a genomic reservoir of regulatory small RNAs. *Embo J*, 31 (20):4005–19, 2012. ISSN 1460-2075 (Electronic) 0261-4189 (Linking). doi: 10.1038/emboj.2012.229.

Muriel Cocaign-Bousquet, Christel Garrigues, Pascal Loubiere, and NicolasD. Lindley. Physiology of pyruvate metabolism in Lactococcus lactis. *Antonie van Leeuwenhoek*, 70(2-4):253–267, 1996. ISSN 0003-6072. doi: 10.1007/BF00395936.

Teresa Cortes, Olga T. Schubert, Graham Rose, Kristine B. Arnvig, Iñaki Comas, Ruedi Aebersold, and Douglas B. Young. Genome-wide Mapping of Transcriptional Start Sites Defines an Extensive Leaderless Transcriptome in Mycobacterium tuberculosis. *Cell Reports*, 5(4): 1121–1131, 09 2014. doi: 10.1016/j.celrep.2013.10.031.

R. Dumoulin, N. Cortes-Perez, S. Gaubert, P. Duhutrel, S. Brinster, R. Torelli, M. Sanguinetti, B. Posteraro, F. Repoila, and P. Serror. Enterococcal Rgg-Like Regulator ElrR Activates Expression of the elrA Operon. *J Bacteriol*, 195(13):3073–83, 2013. ISSN 1098-5530 (Electronic) 0021-9193 (Linking). doi: 10.1128/JB.00121-13.

A. Fouquier d'Hérouël, F. Wessner, D. Halpern, J. Ly-Vu, S. P. Kennedy, P. Serror, E. Aurell, and F. Repoila. A simple and efficient method to search for selected primary transcripts: non-coding and antisense RNAs in the human pathogen Enterococcus faecalis. *Nucleic Acids Res*, 39(7):e46, 2011. ISSN 1362-4962 (Electronic) 0305-1048 (Linking). doi: 10.1093/nar/gkr012.

N. L. Garneau, J. Wilusz, and C. J. Wilusz. The highways and byways of mRNA decay. *Nat Rev Mol Cell Biol*, 8(2):113–26, 2007. ISSN 1471-0072 (Print) 1471-0072 (Linking). doi: 10.1038/nrm2104.

C. Garrigues, P. Loubiere, N. D. Lindley, and M. Cocaign-Bousquet. Control of the shift from homolactic acid to mixed-acid fermentation in Lactococcus lactis: predominant role of the NADH/NAD+ ratio. *J Bacteriol*, 179(17):5282–7, 1997. ISSN 0021-9193 (Print) 0021-9193 (Linking).

M. Golumbeanu. Applying hidden markov models to rna-seq data. http://urn.kb.se/resolve?urn=urn:nbn:se:kth:diva-128384, 2013.

Nancy S. Gutgsell and Chaitanya Jain. Gateway Role for rRNA Precursors in Ribosome Assembly. *Journal of Bacteriology*, 194(24):6875–6882, 2012. doi: 10.1128/JB.01467-12.

N. Innocenti and E. Aurell. Lognormality and oscillations in the coverage of high-throughput transcriptomic data towards gene ends. *J. Stat. Mech*, page P10013, 2013. ISSN 1742-5468. doi: 10.1088/1742-5468/2013/10/P10013.

Jong Hun Kim, Juyoung Lee, Bermseok Oh, Kuchan Kimm, and InSong Koh. Prediction of phosphorylation sites using SVMs. *Bioinformatics*, 20(17):3179–3184, 2004. doi: 10.1093/bioinformatics/bth382.

Louise Kime, Justin E. Clarke, David Romero A., Jane A. Grasby, and Kenneth J. McDowall. Adjacent single-stranded regions mediate processing of tRNA precursors by RNase E direct entry. *Nucleic Acids Research*, 42(7):4577–4589, 2014. doi: 10.1093/nar/gkt1403.

Petr Klus, Simon Lam, Dag Lyberg, Ming Cheung, Graham Pullan, Ian McFarlane, Giles Yeo, and Brian Lam. BarraCUDA - a fast short read sequence aligner using graphics processing units. *BMC Research Notes*, 5(1):27, 2012. ISSN 1756-0500. doi: 10.1186/1756-0500-5-27.

B. Langmead, C. Trapnell, M. Pop, and S. L. Salzberg. Ultrafast and memory-efficient alignment of short DNA sequences to the human genome. *Genome Biol*, 10(3):R25, 2009. ISSN 1465-6914 (Electronic) 1465-6906 (Linking). doi: gb-2009-10-3-r25[pii]10.1186/gb-2009-10-3-r25.

Zhongwei Li, Shilpa Pandit, and Murray P. Deutscher. RNase G (CafA protein) and RNase E are both required for the 5' maturation of 16S ribosomal RNA. *The EMBO Journal*, 18(10): 2878–2885, 1999. ISSN 0261-4189. doi: 10.1093/emboj/18.10.2878.

Sue Lin-Chao, Chia-Li Wei, and Yi-Tzu Lin. RNase E is required for the maturation of ssrA RNA and normal ssrA RNA peptide-tagging activity. *Proceedings of the National Academy of Sciences*, 96(22):12406–12411, 1999. doi: 10.1073/pnas.96.22.12406.

E. Lioliou, C. M. Sharma, I. Caldelari, A. C. Helfer, P. Fechter, F. Vandenesch, J. Vogel, and P. Romby. Global Regulatory Functions of the Staphylococcus aureus Endoribonuclease III in Gene Expression. *PLoS Genetics*, 8(6):e1002782, 2012. ISSN 1553-7404 (Electronic) 1553-7390 (Linking). doi: 10.1371/journal.pgen.1002782.

U Lundberg and S Altman. Processing of the precursor to the catalytic RNA subunit of RNase P from Escherichia coli. *RNA (New York, N.Y.)*, 1(3):327—334, May 1995. ISSN 1355-8382.

George A. Mackie. Determinants in the rpsT mRNAs recognized by the 5'-sensor domain of RNase E. *Molecular Microbiology*, 89(2):388–402, 2013. ISSN 1365-2958. doi: 10.1111/mmi.12283.

E. Matoulkova, E. Michalova, B. Vojtesek, and R. Hrstka. The role of the 3' untranslated region in post-transcriptional regulation of protein expression in mammalian cells. *RNA Biol*, 9(5): 563–76, 2012. ISSN 1555-8584 (Electronic) 1547-6286 (Linking). doi: 10.4161/rna.20231.

Michael L. Metzker. Sequencing technologies – the next generation. *Nat Rev Genet*, 11(1): 31–46, 01 2010.

Taj Morton, Jalean Petricka, David L. Corcoran, Song Li, Cara M. Winter, Alexa Carda, Philip N. Benfey, Uwe Ohler, and Molly Megraw. Paired-End Analysis of Transcription Start Sites in Arabidopsis Reveals Plant-Specific Promoter Signatures. *The Plant Cell Online*, 26 (7):2746–2760, 2014. doi: 10.1105/tpc.114.125617.

P. Nicolas, U. Mader, E. Dervyn, T. Rochat, A. Leduc, N. Pigeonneau, E. Bidnenko, E. Marchadier, M. Hoebeke, S. Aymerich, D. Becher, P. Bisicchia, E. Botella, O. Delumeau, G. Doherty, E. L. Denham, M. J. Fogg, V. Fromion, A. Goelzer, A. Hansen, E. Hartig, C. R. Harwood, G. Homuth, H. Jarmer, M. Jules, E. Klipp, L. Le Chat, F. Lecointe, P. Lewis, W. Liebermeister, A. March, R. A. Mars, P. Nannapaneni, D. Noone, S. Pohl, B. Rinn, F. Rugheimer, P. K. Sappa, F. Samson, M. Schaffer, B. Schwikowski, L. Steil, J. Stulke, T. Wiegert, K. M. Devine, A. J. Wilkinson, J. M. van Dijl, M. Hecker, U. Volker, P. Bessieres, and P. Noirot. Condition-dependent transcriptome reveals high-level regulatory architecture in Bacillus subtilis. *Science*, 335(6072):1103–6, 2012. ISSN 1095-9203 (Electronic) 0036-8075 (Linking). doi: 335/6072/1103[pii]10.1126/science.1206848.

M. B. Pedersen, C. Garrigues, K. Tuphile, C. Brun, K. Vido, M. Bennedsen, H. Mollgaard, P. Gaudu, and A. Gruss. Impact of aeration and heme-activated respiration on Lactococcus lactis gene expression: identification of a heme-responsive operon. *J Bacteriol*, 190(14):4903–11, 2008a. doi: 10.1128/JB.00447-08.

Martin Bastian Pedersen, Christel Garrigues, Karine Tuphile, Celia Brun, Karin Vido, Mads Bennedsen, Henrik Mollgaard, Philippe Gaudu, and Alexandra Gruss. Impact of aeration and heme-activated respiration on Lactococcus lactis gene expression: identification of a heme-responsive operon. *J Bacteriol*, 190(14):4903–4911, Jul 2008b. ISSN 1098-5530 (Electronic); 0021-9193 (Linking). doi: 10.1128/JB.00447-08.

T. Pfeiffer, S. Schuster, and S. Bonhoeffer. Cooperation and competition in the evolution of ATP-producing pathways. *Science*, 292(5516):504–7, 2001. ISSN 0036-8075 (Print) 0036-8075 (Linking). doi: 10.1126/science.1058079.

X. Qin, K. V. Singh, G. M. Weinstock, and B. E. Murray. Characterization of fsr, a regulator controlling expression of gelatinase and serine protease in Enterococcus faecalis OG1RF. *J Bacteriol*, 183(11):3372–82, 2001. ISSN 0021-9193 (Print) 0021-9193 (Linking). doi: 10.1128/JB.183.11.3372-3382.2001.

C. A. Raabe, T. H. Tang, J. Brosius, and T. S. Rozhdestvensky. Biases in small RNA deep sequencing data. *Nucleic Acids Res*, 42(3):1414–26, 2014. ISSN 1362-4962 (Electronic) 0305-1048 (Linking). doi: 10.1093/nar/gkt1021.

S. Rasmussen, H. B. Nielsen, and H. Jarmer. The transcriptionally active regions in the genome of Bacillus subtilis. *Mol Microbiol*, 73(6):1043–57, 2009. doi: 10.1111/j.1365-2958.2009.06830.x.

I. Ruiz de los Mozos, M. Vergara-Irigaray, V. Segura, M. Villanueva, N. Bitarte, M. Saramago, S. Domingues, C. M. Arraiano, P. Fechter, P. Romby, J. Valle, C. Solano, I. Lasa, and A. Toledo-Arana. Base pairing interaction between 5'- and 3'-UTRs controls icaR mRNA translation in Staphylococcus aureus. *PLoS Genet*, 9(12):e1004001, 2013. ISSN 1553-7404 (Electronic) 1553-7390 (Linking). doi: 10.1371/journal.pgen.1004001.

Jan-Philip Schluter, Jan Reinkensmeier, Melanie Barnett, Claus Lang, Elizaveta Krol, Robert Giegerich, Sharon Long, and Anke Becker. Global mapping of transcription start sites and promoter motifs in the symbiotic alpha-proteobacterium Sinorhizobium meliloti 1021. *BMC Genomics*, 14(1):156, 2013. ISSN 1471-2164. doi: 10.1186/1471-2164-14-156.

C. M. Sharma, S. Hoffmann, F. Darfeuille, J. Reignier, S. Findeiss, A. Sittka, S. Chabas, K. Reiche, J. Hackermuller, R. Reinhardt, P. F. Stadler, and J. Vogel. The primary tran-

scriptome of the major human pathogen Helicobacter pylori. *Nature*, 464(7286):250–5, 2010. doi: 10.1038/nature08756.

A. Sittka, S. Lucchini, K. Papenfort, C. M. Sharma, K. Rolle, T. T. Binnewies, J. C. Hinton, and J. Vogel. Deep sequencing analysis of small noncoding RNA and mRNA targets of the global post-transcriptional regulator, Hfq. *PLoS Genet*, 4(8):e1000163, 2008. doi: 10.1371/journal.pgen.1000163.

T.F. Smith and M.S. Waterman. Identification of common molecular subsequences. *Journal of Molecular Biology*, 147(1):195 – 197, 1981. ISSN 0022-2836. doi: http://dx.doi.org/10.1016/0022-2836(81)90087-5.

L. D. Stein, C. Mungall, S. Shu, M. Caudy, M. Mangone, A. Day, E. Nickerson, J. E. Stajich, T. W. Harris, A. Arva, and S. Lewis. The generic genome browser: a building block for a model organism system database. *Genome Res*, 12(10):1599–610, 2002. ISSN 1088-9051 (Print) 1088-9051 (Linking). doi: 10.1101/gr.403602.

A. Toledo-Arana, O. Dussurget, G. Nikitas, N. Sesto, H. Guet-Revillet, D. Balestrino, E. Loh, J. Gripenland, T. Tiensuu, K. Vaitkevicius, M. Barthelemy, M. Vergassola, M. A. Nahori, G. Soubigou, B. Regnault, J. Y. Coppee, M. Lecuit, J. Johansson, and P. Cossart. The Listeria transcriptional landscape from saprophytism to virulence. *Nature*, 459(7249):950–6, 2009. doi: 10.1038/nature08080.

C. Trapnell, B. A. Williams, G. Pertea, A. Mortazavi, G. Kwan, M. J. van Baren, S. L. Salzberg, B. J. Wold, and L. Pachter. Transcript assembly and quantification by RNA-Seq reveals unannotated transcripts and isoform switching during cell differentiation. *Nat Biotechnol*, 28 (5):511–5, 2010. ISSN 1546-1696 (Electronic) 1087-0156 (Linking). doi: 10.1038/nbt.1621.

Johannes H Urban and Jorg Vogel. Two seemingly homologous noncoding RNAs act hierarchically to activate glmS mRNA translation. *PLoS Biol*, 6(3):e64, Mar 2008. ISSN 1545-7885 (Electronic); 1544-9173 (Linking). doi: 10.1371/journal.pbio.0060064.

Oliver Vesper, Shahar Amitai, Maria Belitsky, Konstantin Byrgazov, Anna Chao Kaberdina, Hanna Engelberg-Kulka, and Isabella Moll. Selective Translation of Leaderless mRNAs by Specialized Ribosomes Generated by MazF in Escherichia coli. *Cell*, 147(1):147 – 157, 2011. ISSN 0092-8674. doi: http://dx.doi.org/10.1016/j.cell.2011.07.047.

E. G. Wagner and J. Vogel. *Approaches to identify Novel Non-messenger RNAs in Bacteria and to investigate their Biological Functions: Functional Analysis of Identified Non-mRNAs.* Wiley-VCH Verlag GmbH & Co., KGaA Weinheim, 2005.

L. Winstedt, L. Frankenberg, L. Hederstedt, and C. von Wachenfeldt. Enterococcus faecalis V583 contains a cytochrome bd-type respiratory oxidase. *J Bacteriol*, 182(13):3863–6, 2000. ISSN 0021-9193 (Print) 0021-9193 (Linking). doi: 10.1128/JB.182.13.3863-3866.2000.

V Yajnik and G N Godson. Selective decay of Escherichia coli dnaG messenger RNA is initiated by RNase E. *Journal of Biological Chemistry*, 268(18):13253–13260, 1993.

Y. Yamamoto, C. Poyart, P. Trieu-Cuot, G. Lamberet, A. Gruss, and P. Gaudu. Roles of environmental heme, and menaquinone, in Streptococcus agalactiae. *Biometals*, 19(2):205–10, 2006. doi: 10.1007/s10534-005-5419-6.
